# Supplementary material for: Recent Advances in RecBole: Extensions with more Practical Considerations
Source: arXiv:2211.15148 source file (2022-11-28)
Supplement: Supplementary file 1 [file sec-appendix.tex]

\section{APPENDIX}

\begin{figure}[hb]
    \centering
    \lstinputlisting[language=python]{figs/ddp.py}
    \caption{Usage example of Distributed Training}
    \label{fig:ddp}
\end{figure}

\begin{figure}[hb]
    \lstinputlisting[language=python]{figs/hyper-example.py}
    \caption{Usage examples of two hyper-tuning tools.}\label{fig:hyper-example}
\end{figure}

\begin{figure}[hb]
    % \flushleft 
    \subfigure[Grid Search]{%
        \lstinputlisting[language=python]{figs/grid.py}
        \label{fig:grid}
    }
    \subfigure[Random Search]{%
        \lstinputlisting[language=python]{figs/random.py}
        \label{fig:random}
    }
    \subfigure[Bayesian Hyper-opt]{%
        \lstinputlisting[language=python]{figs/bayes.py}
        \label{fig:bayes}
    }
    \caption{Usage examples of hyper-tuning strategies.}
    \label{fig:hyper-opt}
\end{figure}
